# Supplementary material for: Can a Suit of Armor Conduct Electricity? A New Dataset for Open Book Question Answering
Source: arXiv:1809.02789 source file (2018-09-08)
Supplement: Supplementary file 1 [file supplement.tex]

%
% File emnlp2018.tex
%
%% Based on the style files for EMNLP 2018, which were
%% Based on the style files for ACL 2018, which were
%% Based on the style files for ACL-2015, with some improvements
%%  taken from the NAACL-2016 style
%% Based on the style files for ACL-2014, which were, in turn,
%% based on ACL-2013, ACL-2012, ACL-2011, ACL-2010, ACL-IJCNLP-2009,
%% EACL-2009, IJCNLP-2008...
%% Based on the style files for EACL 2006 by 
%%e.agirre@ehu.es or Sergi.Balari@uab.es
%% and that of ACL 08 by Joakim Nivre and Noah Smith

\documentclass[11pt,a4paper]{article}
\usepackage[table,dvipsnames]{xcolor} % Needs to be here to avoid clashes with other packages
\usepackage[hyperref]{emnlp2018}
\usepackage{times}
\usepackage{latexsym}
\usepackage{adjustbox}

\usepackage{url}

\aclfinalcopy % Uncomment this line for the final submission
\def\aclpaperid{2133} %  Enter the acl Paper ID here

%\setlength\titlebox{5cm}
% You can expand the titlebox if you need extra space
% to show all the authors. Please do not make the titlebox
% smaller than 5cm (the original size); we will check this
% in the camera-ready version and ask you to change it back.

\newcommand\BibTeX{B{\sc ib}\TeX}
\newcommand\confname{EMNLP 2018}
\newcommand\conforg{SIGDAT}

\usepackage{amsmath}
\usepackage{amsthm}
\usepackage{amsfonts}
\usepackage{color}
\usepackage{enumitem}
\usepackage{xspace}
\usepackage{booktabs,colortbl}
\usepackage{array}
\input{macros}

\title{Supplement to paper ``Can a Suit of Armor Conduct Electricity?\\
A New Dataset for Open Book Question Answering''
}

\author{
Todor Mihaylov$^\ddagger$ \and Peter Clark$^\dagger$ \and Tushar Khot$^\dagger$ \and Ashish Sabharwal$^\dagger$\\
\\
$^\dagger$ Allen Institute for Artificial Intelligence, Seattle, WA, U.S.A.\\
%$^\ddagger$ Dept.\ of Computational Linguistics, Heidelberg University, Heidelberg, Germany\\
$^\ddagger$ Research Training Group AIPHES \& Heidelberg University, Heidelberg, Germany\\
{\tt \small \{peterc,tushark,ashishs\}@allenai.org, mihaylov@cl.uni-heidelberg.de}
}

\date{}

\begin{document}

\maketitle

\input{appendix}

\bibliographystyle{acl_natbib_nourl}
\bibliography{open-book-qa}

\end{document}
